# Supplementary material for: FORUM: Frozen Outputs Reconciled Using Model Agreement for Visual Grounding
Source: arXiv:2609.37488 source file (2026-09-27)
Supplement: Supplementary file 1 [file supp_titlepage.tex]

% Supplementary title block. Shared by supp.tex (standalone submission build)
% and the optional single-PDF review block in main.tex.
\begin{center}
  {\Large\bfseries \PaperTitleEN\par}
  \vspace{4pt}
  {\Large\bfseries Supplementary Material\par}
  \vspace{22pt}
  Taiyo Sato, Takamasa Sanda, Keisuke Maeda, Takahiro Ogawa, Miki Haseyama, and Shunya Nagashima\par
\end{center}
\vspace{18pt}
